# Supplementary material for: A Non-Linear Kalman Filter for track parameters estimation in High Energy Physics
Source: arXiv:2112.09470 source file (2021-12-17)
Supplement: Supplementary file 1 [file Supplementary_Material.pdf]

1 **Supplementary Material for**

2 **A Non-Linear Kalman Filter for track parameters esCtimation in High Energy Physics**

3 **Xiaocong Ai, Heather M. Gray, Andreas Salzburger and Nicholas Styles**

4 **Corresponding author: Xiaocong Ai**

5 **E-mail: [xiaocong.ai@desy.de](mailto:xiaocong.ai@desy.de)**

6 **This PDF file includes:**

7 Figs. S1 to S3 (not allowed for Brief Reports)

## 8 Supplementary Figures

9 The distributions of residual mean, residual RMS and pull RMS for those track parameters not shown in the manuscript are  
10 included here.

11 **Distributions of residual mean and RMS.** Fig. S1 shows the mean of the residuals of the track parameters  $\phi$ ,  $\theta$ ,  $q/p$  and  $t$  as a  
12 function of  $\eta$  for simulated particles with  $p_T > 20$  GeV. Fig. S2 shows the RMS of the residuals of the track parameters  $\phi$ ,  $\theta$ ,  
13  $q/p$  and  $t$  as a function of  $\eta$  for simulated particles with  $p_T > 20$  GeV.

14 **Distributions of pull RMS.** Fig. S3 shows the RMS of the pulls of the track parameters  $\phi$ ,  $\theta$ ,  $q/p$  and  $t$  as a function of  $p_T$  for  
15 simulated particles with  $1.0 < |\eta| < 2.5$ .

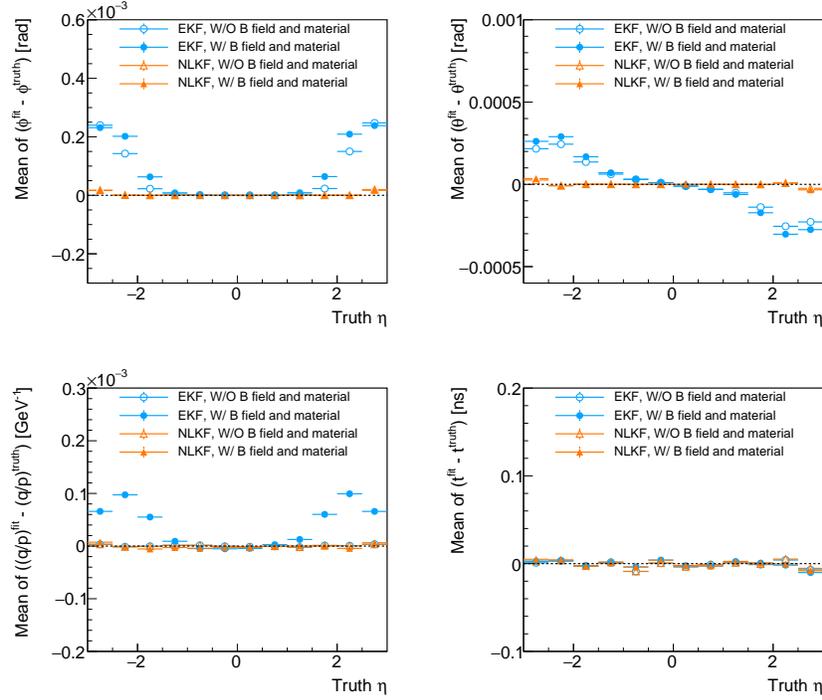

**Fig. S1.** The mean of the residual of fitted perigee track parameters  $\phi$ ,  $\theta$ ,  $q/p$  and  $t$  parameterized as a function of simulated particle  $\eta$  ( $20 < p_T < 100$  GeV) for the ODD without (blue circles for EKF, orange hollow triangles for NLKF) and with (blue dots for EKF, orange filled triangles for NLKF) the presence of a solenoidal magnetic field of 2 T and material effects. The dashed horizontal lines in the upper panel denote the expected mean of the residuals.

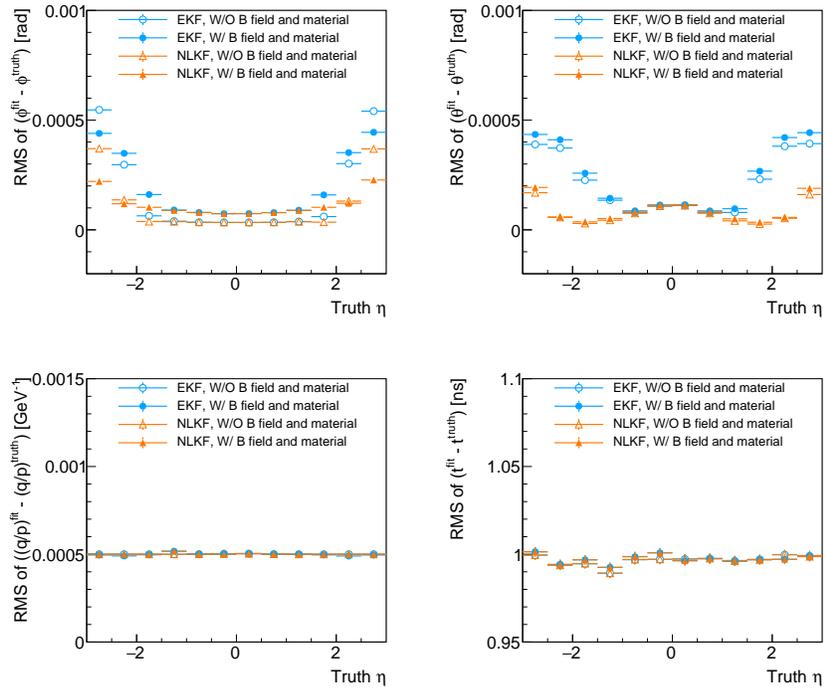

**Fig. S2.** The RMS of the residual of fitted perigee track parameters  $\phi$ ,  $\theta$ ,  $q/p$  and  $t$  parameterized as a function of simulated particle  $\eta$  ( $20 < p_T < 100$  GeV) for the ODD without (blue circles for EKF, orange hollow triangles for NLKF) and with (blue dots for EKF, orange filled triangles for EKF) the presence of a solenoidal magnetic field of 2T and material effects.

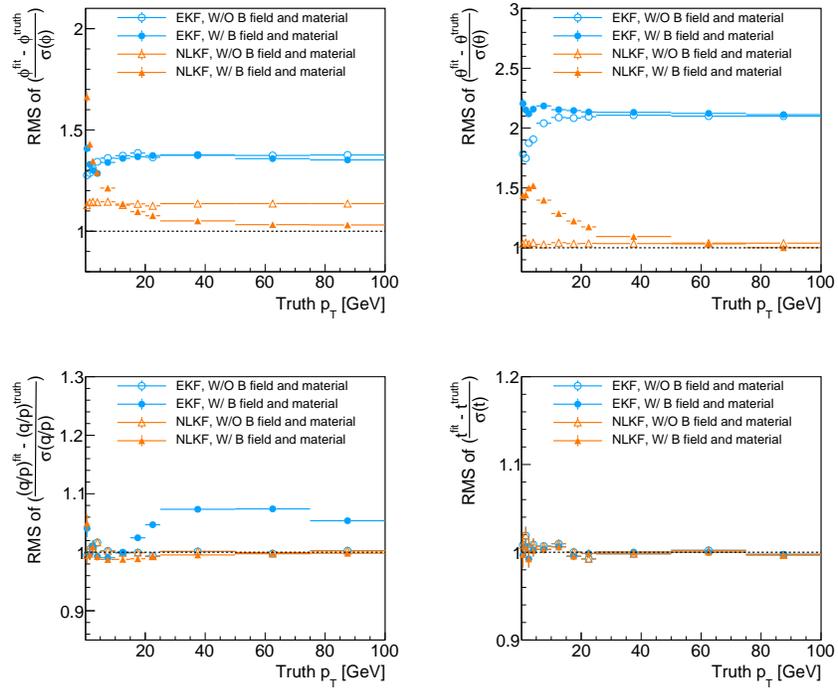

**Fig. S3.** The RMS of the pull of fitted perigee track parameters  $\phi$ ,  $\theta$ ,  $q/p$  and  $t$  parameterized as a function of simulated particle  $p_T$  ( $1.0 < |\eta| < 2.5$ ) for the ODD without (blue circles for EKF, orange hollow triangles for NLKF) and with (blue dots for EKF, orange filled triangles for EKF) the presence of a solenoidal magnetic field of 2 T and material effects. The dashed horizontal lines denote the expected RMS of the pulls.
